# Supplementary material for: An Unbiased Transformer Source Code Learning with Semantic Vulnerability Graph
Source: arXiv:2304.11072 source file (2023-04-17)
Supplement: Supplementary file 1 [file 7_appendix.tex]

\color{red}

\section{Ablation studies on PF Rich Sample Programs}
When we analyzed the ablation studies of our PF edges, we saw a moderate (2-3\%) improvement in the evaluation metrics. Since this is a marginal improvement over the previous metrics, we dug deeper to understand the impact of our PF edges. We analyzed the datasets we used for our experiments and found that only around 10\% of the code samples are suitable for PF edges. In other words, we can generate PF edges from only 10\% of source codes. Hence we created some sample programs that are rich in PF edges. We collected 144 sample PF edge-rich programs (vulnerable and non-vulnerable) and compared our work with publicly available models (Devign \cite{zhou2019devign}, VELVET \cite{ding2021velvet}). These 144 examples were never used for training but only for testing purposes. Moreover, we also implemented $\mu$VulDeePecker \cite{zou2019mu} based on their architecture for comparison. Since these programs have more PF edges, our model has an advantage in detecting vulnerabilities for these sample programs. Table \ref{tab:appendix_1} Show the CWE numbers, numbers of PF edges and how many vulnerable and non-vulnerable examples we compiled.

% Please add the following required packages to your document preamble:
% \usepackage{booktabs}
\begin{table}[ht]
\centering
\caption{\color{red} An Ablation Study on the effect on PF Rich Sample Programs on 144 Vulnerable and Non-Vulnerable Programs\color{black}}
\label{tab:appendix_1}
\begin{tabular}{p{0.08\textwidth}
                 p{0.03\textwidth}
                 p{0.03\textwidth}
                 p{0.03\textwidth}
                 p{0.08\textwidth}
                 p{0.12\textwidth}}
\toprule
CWE                                                           & DP & AC & RM & Vulnerable & Non-Vulnerable \\ \midrule
CWE-601 & 10 & 8  & 10 & 5          & 5              \\
CWE-863                              & 10 & 7  & 9  & 5          & 4              \\
CWE-602 & 11 & 3  & 6  & 5          & 5              \\
CWE-441 & 12 & 7  & 14 & 5          & 5              \\
CWE-799  & 4  & 5  & 6  & 3          & 3              \\
CWE-352 & 1  & 8  & 0  & 3          & 3              \\
CWE-131   & 9  & 0  & 2  & 3          & 3              \\
CWE-134       & 10 & 0  & 4  & 5          & 5              \\
CWE-197   & 10 & 0  & 0  & 4          & 4              \\
CWE-252 & 8  & 0  & 0  & 6          & 2              \\
CWE-481 & 1  & 8  & 4  & 3          & 3              \\
CWE-617 & 6  & 0  & 3  & 3          & 3              \\
CWE-788 & 6  & 8  & 4  & 3          & 3              \\
CWE-338 & 9  & 0  & 0  & 4          & 5              \\
CWE-415 & 0  & 0  & 8  & 4          & 4              \\
CWE-457& 12 & 0  & 0  & 4          & 4              \\
CWE-571& 5  & 0  & 0  & 2          & 3              \\
CWE-690 & 6  & 6  & 0  & 3          & 3              \\ \midrule
                                                              &    &    &    & \multicolumn{2}{l}{Total = 144} \\ \bottomrule

\end{tabular}
\end{table}

Our experimental results show that out of the 144 examples, our model detects 140 correctly, achieving an accuracy of 97\%. Devign, VELVET, and $\mu$VulDeePecker achieved an accuracy of 81\%, 79\%, and 64\%, respectively, improving the performance of our model by almost 16\%

\color{black}
